# Supplementary material for: Adaptive stochastic Galerkin FEM for lognormal coefficients in hierarchical tensor representations
Source: arXiv:1811.00319 source file (2018-11-01)
Supplement: Supplementary file 1 [file appendix.tex]

\subsection{TT residual decomposition}
\label{sec:tt-residual-decomposition}
\todo{\tiny introduction}

A low rank representation of the residual~\eqref{eq:residual} can be derived by
\begin{align}
\mathcal R_+(w_N) &= f-\mathcal A_+(w_N) = f - \nabla \cdot (a_+ \nabla w_N) \\
&=f - \nabla \cdot \left( \sum_{i,j=1}^{N,K} \sum_{\nu \in \Delta} \sum_{\mu \in \Lambda} R(j,\nu) W(i,\mu) \psi_j \nabla \phi_i \Hthrh_\nu \Hthrh_\mu \right) \\
&= f - \Biggl( \sum_{k_1' = 1}^{s_1} \cdots \sum_{k_L' = 1}^{s_L} \sum_{k_1 = 1}^{r_1} \cdots \sum_{k_M = 1}^{r_M} \biggl( \sum_{i,j=1}^{N,K} R_0(j,k_1') W_0(i,k_1) \nabla \cdot (\psi_j \nabla \phi_i) \biggr) \\
&\qquad\qquad \times \prod_{m=1}^M \biggl( \sum_{\nu_m = 0}^{q_m-1} \sum_{\mu_m = 0}^{d_m-1} \sum_{\eta_m = 0}^{\min(\nu_m,\mu_m)} R_m(k_m',\nu_m,k_{m+1}') W_m(k_m,\mu_m,k_{m+1}) \\
&\qquad\qquad\qquad\qquad \tilde\kappa_{\nu_m,\mu_m}^{\eta_m} \Hthrh_{\nu_m + \mu_m - 2 \eta_m} \biggr) \\
&\qquad\qquad \prod_{\ell=M+1}^L \biggl( \sum_{\nu_\ell = 0}^{q_\ell-1} R_l(k_\ell',\nu_\ell,k_{\ell+1}') \Hthrh_{\nu_\ell} \biggr) \Biggr) .
\end{align}
This generates a TT tensor $S$ of order $L$ in the following way:
For the first component we get
\begin{equation}
S_0(p,k_1'') \chi_p = R_0(j,k_1') S_0(i,k_1) \psi_j \nabla \phi_i,\quad \text{with} \; \nabla \cdot\chi_p = \nabla\cdot (\psi_j\nabla\phi_i)
\end{equation}
using the index bijections
\begin{align}
p &\leftrightarrow (i,j), \ p = 1,\ldots,P=NK, \\
k_1'' &\leftrightarrow (k_1',k_1), \ k_1'' = 1,\ldots,t_1=s_1 r_1.
\end{align}
For $m = 1,\ldots,M$, we have to solve the equations
\begin{align}
\sum_{\nu_m=0}^{q_m-1} \sum_{\mu_m=0}^{d_m-1} &\sum_{\eta_m = 0}^{\min(\nu_m,\mu_m)} R_m(k_m',\nu_m,k_{m+1}') W_{m}(k_m,\mu_m,k_{m+1}) \tilde\kappa_{\nu_m,\mu_m}^{\eta_m} \Hthrh_{\nu_m + \mu_m - 2 \eta_m} \\
&= \sum_{\xi_m=0}^{q_m+d_m-2} S_m(k_m'',\xi_m,k_{m+1}'') H_{\xi_m}^{\tau_{\theta\rho}}
\end{align}
with index bijections
\begin{align}
k_m'' &\leftrightarrow (k_m',k_m), \ k_m'' = 1,\ldots,t_m=s_m r_m, \\
k_{m+1}'' &\leftrightarrow (k_{m+1}',k_{m+1}), \ k_{m+1}'' = 1,\ldots,t_{m+1}=s_{m+1} r_{m+1}
\end{align}
and dimensions $z_m = d_m + q_m + 1$.
\todo{\tiny define $r_0=r_{M+1}=0$ in ALS algorithm as solution rank}
This can be done with a simple matrix multiplication
\begin{equation}
S_m(k_m'',\xi_m,k_{m+1}'') = \sum_{\nu_m=0}^{q_m-1} \sum_{\mu_m=0}^{d_m-1} R_m(k_m',\nu_m,k_{m+1}') W_m(k_m,\mu_m,k_{m+1}) \kappa_{\nu_m,\mu_m}^{\xi_m},
\end{equation}
where $\kappa_{\nu_m,\mu_m}^{\eta_m}$ is defined as in \eqref{eq:betacoeffs}.
Finally, the remaining components $S_\ell, \ell=M+1,\ldots,L$ are simply given as
\begin{equation}
S_\ell(k_\ell'',\xi_l,k_{\ell+1}'') H_{\xi_\ell}^{\tau_{\theta\rho}} = R_l(k_\ell',\xi_\ell,k_{\ell+1}') H_{\xi_\ell}^{\tau_{\theta\rho}},
\end{equation}
where the index bijections are identities and the dimensions are $z_\ell = q_\ell$.
The resulting stochastic set is 
\begin{align}
\Xi &:= \bigl\{ \xi = (\xi_1,\ldots,\xi_L)\; |\; \xi_m = 0,\ldots,z_m-1, m = 1,\ldots,M; \xi_l = 0,\ldots,z_\ell-1,\\ 
& \ell = M+1,\ldots,L \bigr\} =: \Xi_1 \times \ldots \times \Xi_L \times \ldots.
\end{align}
The preceding derivations lead to a TT decomposed of the residual of the form
\begin{align}
	\mathcal R_+(w_N) &= f - \sum_{k_1''}^{t_1} \cdots \sum_{k''_L}^{t_L} \bigl( \sum_p^{NK} S_0(p,k_1'') \nabla \cdot \chi_p \bigr) \bigl( \sum_{\eta_1=0}^{z_1-1''} S_1(k_1'',\eta_1,k_2'') \Hthrh_{\eta_1} \bigr) \times
	\\&  \quad \times \cdots \times \bigl( \sum_{\eta_L=0}^{Z_L-1''} S_L(k_L'',\eta_L) \Hthrh_{\eta_L} \bigr)
\end{align}
Thus, we can write 
\begin{equation}
	\mathcal R_+(w_N) = 
	%\sum_{\xi \in \Xi} r_\mu(w_N) H_\mu = 
	% I do not think we need the formulation with r_\mu. We already have the expression in Hermite polynomials and developing them again will only change f, s.t. it depends on \mu as well. This can be seen directly.
	f- \sum_{p=1}^P \sum_{\xi \in \Xi} S(p,\xi) \nabla \cdot \chi_p \Hthrh_\xi .
\end{equation}

With $f$ beeing independent of the stochastic and the decomposition of the index set and the splitting~\eqref{eq:residualSplit}, it follows
\begin{align}
\label{eq:residualSplit}
\mathcal R_+(w_N) &= \mathcal R_\Lambda(w_N) + \mathcal R_{\Xi \setminus \Lambda}(w_N), \\
\label{eq:LambdaResidual}
\mathcal R_\Lambda(w_N) &= f\delta_{\mu, 0} - \sum_{j=1}^K\sum_{i=1}^N \sum_{\mu \in \Lambda} S(j,i,\mu) \nabla \cdot \psi_j\nabla\phi_i \Hthrh_\mu, \\
\mathcal R_{\Xi \setminus \Lambda}(w_N) &= - \sum_{j=1}^K\sum_{i=1}^N \sum_{\mu \in \Xi \setminus \Lambda} S(j,i,\mu) \nabla \cdot \psi_j\nabla\phi_i \Hthrh_\mu
\end{align}
for some coefficient tensor $S\in\bbR^{K,N,d_1+q_1, \ldots, d_M+q_M,q_{M+1},\ldots, q_L}$ given in compressed tensor train format as described above.

%%%%%%%%%%
This leads to an explicit form for the error estimators as summarized in the following lemma.

\begin{lemma}
  \label{lem:active estimator}
  Assume $w_N\in\mcV_p(\Lambda,\mcT)$, $v\in\mcV_{\theta\rho}$, $\mathcal Q$ as in~\eqref{eq:clement} and set
  \begin{align}
    \eta_T(w_N) &:= \int_T\int_\Gamma \zeta_{\theta\rho}^2\left(\sum_{\mu\in\Lambda}f\delta_{\mu,0} + \sum_{p=1}^P S(p,\mu)\nabla\cdot\chi_p\Hthrh_\mu\right)^2\dx{\gamma}(y)\dx{x},\\
    \eta_F(w_N) &:=  \int_T\int_\Gamma \zeta_{\theta\rho}^2\left(\jump{\sum_{p=1}^P \sum_{\mu\in\Lambda} S(p,\mu)\chi_p\Hthrh_\mu}_S \right)^2\dx{\gamma}(y)\dx{x}.
  \end{align}
  Then, it holds
  \begin{equation}
    \langle R_{\Lambda}(w_N), v-Qv \rangle \lesssim \left\{\sum_{T\in\mcT} h_T\eta_T(w_N) + \sum_{F\in\mcF}h_F^{1/2}\eta_F(w_N)\right\}\norm{v}_{L^2(\Gamma,\gamma;\mcX)}.
  \end{equation}
\end{lemma}
\begin{proof}
  Inserting the residual~\eqref{eq:LambdaResidual} and the weight~\eqref{eq:newWeight} in the estimation of~\eqref{eq:residualEstimate} and using the interpolation estimate~\eqref{eq:clement} proves the claim.

\end{proof}

\begin{lemma}
  \label{lem:inactive estimator}
  For $w_N\in\mcV_p(\Lambda,\mcT)$, $v\in\mcV_{\theta\rho}$ and $\mathcal Q$ as in~\eqref{eq:clement} it holds
  \begin{equation}
    \langle R_{\Xi\setminus\Lambda}(w_N), v\rangle \lesssim \Theta(w_N)\norm{v}_{L^2(\Gamma,\gamma;\mcX)},
  \end{equation}
  where
  \begin{equation}
    \Theta(w_N)^2 := \int_T\int_\Gamma \zeta_{\theta\rho}^2\left(\sum_{\mu\in\Xi\setminus\Lambda}\sum_{p=1}^P S(p,\mu)\chi_p\Hthrh_\mu\right)^2\dx{\gamma}(y)\dx{x}.
  \end{equation}
\end{lemma}
\begin{proof}
  By definition of the inactive residual part it holds
  \begin{align}
	\langle R_{\Xi\setminus\Lambda}(w_N), v\rangle =  \int_D\int_\Gamma \left(-\sum_{p=1}^P\sum_{\mu\in\Xi\setminus\Lambda} S(p,\mu)\chi_p \Hthrh_\mu\right)\nabla v \dx{\gammatr}(y)\dx{x}.
  \end{align}
  The claim follows by employing the weight $\zeta_{\theta\rho}$, the Cauchy-Schwarz inequality and the usual Sobolev embedding.
  \todo{\tiny Sobolev? embedding of the weighted spaces?}
\end{proof}

\subsection{Numerical treatment}
%TODO: add weight as an rank one operator
% or argue with it as a constant
For each element $T \in \mathcal T$, we define the residual estimator component
\begin{align}
\eta_T(w_N)^2 &= \int_T \int_\Gamma\zeta_{\theta\rho}^2 \Biggl(\sum_{\mu \in \Lambda}f\delta_{\mu, 0} + \sum_{p=1}^P S(p,\mu) \nabla \cdot \chi_p \Hthrh_\mu \Biggr)^2 \dx{\gamma}(y) \dx{x} \\
& = \int_T f^2\dx{x} + 2\sum_{\mu\in\Lambda}\sum_{p=1}^P S(p,\mu)\int_T \nabla\cdot\chi_p f\delta_{\mu,0} \dx{x}\int_\Gamma\zeta_{\theta\rho}^2 \Hthrh_\mu \dx{\gamma}(y) \\
 &\qquad + \sum_{\mu\in\Lambda}\sum_{\mu'\in\Lambda}\sum_{p=1}^P\sum_{p'=1}^P S(p,\mu)S(p',\mu')\int_T \Bigl( \nabla \cdot \chi_p \Bigr) \Bigl( \nabla \cdot \chi_{p'} \Bigr) \dx{x}\\
 &\qquad\qquad \int_\Gamma \Hthrh_\mu \Hthrh_{\mu'} \zeta_{\theta\rho}^2\dx{\gamma}(y) 
\end{align}
A downside of the change of the measure to $\gamma$ and the involved weight $\zeta_{\theta\rho}^2$ is the fact that the shifted hermite polynomials are not orthogonal under this measure. 
However, this can property can be restored easily by calculating the basis change integrals beforehand.
This results in a rank-one operator $\mathbf H$ that can be inserted in order to calculate the scalar product:
\begin{align}
\mathbf H_T(p,p';\xi_1,\xi_1';\ldots;\xi_L,\xi_L') &= H_T(p,p') \otimes H_1(\xi_1,\xi_1') \otimes \ldots \otimes H_L(\xi_L,\xi_L'), \\
H_T(p,p') &= \int_T \Bigl( \nabla \cdot \chi_p \Bigr) \Bigl( \nabla \cdot \chi_{p'} \Bigr) \dx{x}, \\
H_\ell(\xi_\ell,\xi_\ell') &= \int_{\Gamma} \zeta_{\theta\rho}^2 \Hthrh_{\xi_\ell} \Hthrh_{\xi_\ell'}  \mathrm{d}\gamma(y_\ell), \qquad \ell = 1,\ldots,L .
\end{align}
Finally, the estimator takes the form
\begin{align}
\eta_T(w_N)^2 &= \int_T f^2\dx{x} + 2\sum_{p=1}^P \tilde{S}(p,0,\ldots, 0)\int_T \nabla\cdot\chi_p f \dx{x} %\int_\Gamma H_0 \dx{\gamma}(y)
 \\
%  &\qquad + \sum_{\mu\in\Lambda}\sum_{\mu'\in\Lambda}\sum_{p=1}^P\sum_{p'=1}^P S(p,\mu)S(p',\mu')\int_T \Bigl( \nabla \cdot \chi_p \Bigr) \Bigl( \nabla \cdot \chi_{p'} \Bigr) \dx{x}\int_\Gamma H_\mu H_{\mu'} \dx{\gamma}(y)
&\qquad + \sum_{\mu\in\Lambda}\sum_{p=1}^P\sum_{p'=1}^P \tilde{S}(p,\mu)\tilde{S}(p',\mu)\int_T \Bigl( \nabla \cdot \chi_p \Bigr) \Bigl( \nabla \cdot \chi_{p'} \Bigr) \dx{x},
\end{align}
where $\tilde{S} = H\circ S$, denoting the matrix-vector multiplication of every component of the operator $H$ with the corresponding component of the tensor train $S$.
%The existence of $\norm{H_\mu H_{\mu'}}_{L^2(\Gamma,\gamma_\rho)}$ can be shown by the recursive relation~\eqref{eq:recursionym} or directly by the observation in Lemma~\ref{lem:tripleH} together with the embedding~\eqref{eq:embedding}.

Similarly, for the jump over the edge $F$ we obtain the estimator
\begin{align}
  \eta_F(w_N)^2 &= \sum_{\mu\in\Lambda}\sum_{p=1}^P\sum_{p'=1}^P \tilde{S}(p,\mu)\tilde{S}(p',\mu)\int_F \jump{\nabla \cdot \chi_p \nabla \cdot \chi_{p'} }
\end{align}

Resulting from the elaborated ideas for the tail estimator in~\eqref{eq:tailestimatorCont} we obtain a decomposition of the estimator in lemma~\ref{lem:inactive estimator} for every dimension $n=1,2,\ldots$ using the sets~\eqref{eq:Deltan}.
For every $n=1,2,\ldots$ and $w_N\in\mcV_p(\Lambda, \mcT)$ we define 
\begin{align*}
  \Theta_n(w_N)^2 &= \int_D\int_\Gamma \zeta_{\theta\rho}^2\Bigl(-\sum_{\nu\in\Delta_N}\sum_{p=1}^P S(p,\nu)\chi_p\Hthrh_\nu\Bigr)^2 \dgam{y}\dx{x}.
\end{align*}
Using the same arguments and notation as above, we can simplify
\begin{align*}
  \Theta_n(w_N)^2 &= \sum_{\nu\in\Delta_n}\sum_{p=1}^P\sum_{p'=1}^P\tilde{S}(p,\nu)\tilde{S}(p',\nu)\int_D\chi_p\cdot\chi_{p'}\dx{x}.
\end{align*}
\begin{remark}
All the involved summations can be computated efficiently due to the tensor train format.
\end{remark}
%\todo{\tiny the main term can be computed now. the consistency $\norm{u_N-w_N}$ should be as in [EPS] based on the TT residual. for the last $\mcA_-$ term, some new ideas have to be employed.}

% Thus, we chose $\theta := \min_{m=\mathbb N}\Bigl( \frac{1}{4\rho \alpha_m} \Bigr)$ and obtain
% \begin{equation}
% \exp{2\theta \rho \alpha_m} < \exp{1/2} < 2.
% \end{equation}

% Theoretically, the matrix product operator can thus be reproduced exactly on this space, but storage would grow exponentially with $M$. A low rank approximation is crucial. For the evaluation of the error
% that is due to this low rank approximation, we can exploit basic ideas from linear algebra, which will be done later. An additional error in the operator is the result of the midpoint-discretization of the deterministic part of the coefficient.
% This is akin to errors that result from quadrature and numerical integration.
%
% The error that occurs due to the restriction of the solution space should be split in three ways: First, we have introduced a FEM-discretization of the domain $D$; secondly, we have restricted the number of factors in the coefficient $M$
% and the degree of the generalized polynomial chaos discretization; and thirdly, the solution also requires a low rank approximation due to the exponential growth of the coefficient tensor $V$.
