# Supplementary material for: Adaptive stochastic Galerkin FEM for lognormal coefficients in hierarchical tensor representations
Source: arXiv:1811.00319 source file (2018-11-01)
Supplement: Supplementary file 2 [file appendix_old.tex]

\section{problem-dependent space}

\textcolor{blue}{ We rather need something like:
\begin{align}
\label{eq:clement}
  \begin{array}{rlr}
    \norm{e^{\frac{a}{2}}(v-\mcI v)}_{L^2(\Gamma, \gamma_\rho; L^2(T))} &\lesssim h_T\norm{v}_{\mcA_+} &\text{for } T\in\mcT
  \end{array}\\
\end{align}
what we might not get. 
The problem is, we can not simply get rid of $e^a$, since we need it for the energy norm and if we use the standard Clement operator proof to obtain an upper bound we only get 
\begin{equation}
  \norm{e^{\frac{a}{2}}(v-\mcI v)}_{L^2(\Gamma, \gamma_\rho; L^2(T))} = \int_\Gamma \norm{e^{\frac{a}{2}}(v-\mcI v)}_{L^2(T)} \mathrm{d}\gamma_\rho \lesssim h_T \int_\Gamma \norm{\nabla e^{\frac{a}{2}}(v-\mcI v)}_{L^2(T)} \mathrm{d}\gamma_\rho
\end{equation}
where the gradient acts on $e^a$ as well. 
So, we need: 
\begin{equation}
\norm{\nabla e^{\frac{a}{2}}(v-\mcI v)}_{L^2(T)} \leq \norm{e^{\frac{a}{2}}\nabla(v-\mcI v)}_{L^2(T)}.
\end{equation}
Otherwise, we need to consider the idea of Max, going away from the energy norm, again.
Maybe we can use Martin's equivalence of the weighted $L^2$ norms? 
}

\textcolor{green}{ME: That's a valid point. However, (3.38) and (3.39) are not correct. In particular, the gradient usually is the bound of the interpolation error.\\[1ex]
Rough (somewhat incorrect) sketch of a suggestion, looking at the terms we want to cancel out ($R$ is the residual leading to the actual FE estimator):
\begin{align}
  \frac{\int_\Gamma \norm{e^{a/2}R(1-\mcI)v}_{L^2(D)}^2\dx{\gamma_{\theta\rho}}}{\int_\Gamma \norm{e^{a/2} \nabla v}_{L^2(D)}^2\dx{\gamma_{\theta\rho}}} &\leq \frac{\norm{e^{a/2}\frac{\zeta_{\theta\rho}}{\zeta_\rho}}_{L^\infty(\Gamma)}\int_\Gamma \norm{R}_{L^2(D)}^2 \zeta_\rho^2\dx{\gamma}\int_\Gamma \norm{v}_\mcX^2 \dx{\gamma}}{\check c \int_\Gamma\norm{v}_\mcX^2\dx{\gamma}}\\
  &\leq \frac{\hat c \norm{\zeta_\rho^2}_{L^\infty(\Gamma)}}{\check c} \int_\Gamma \norm{R}_{L^2(D)}^2 \dx{\gamma_\rho}.
\end{align}
The first inequality separates $(1-\mcI)v$ and consequently leads to the required interpolation bound $\abs{\nabla v}$.
Note that $\mcI$ here is supposed to be something like the Cl\'ement interpolation in all stochastic components, i.e. $\int_\Gamma \norm{(1-\mcI)v H_\nu}_{L^2(D)}\dx{\gamma} \leq \norm{v_\nu}_\mcX$ for $\nu\in\Lambda$.
To cancel with the denominator, we can factorize a lower bound $\check c$ of $e^{a/2}$ and obtain the integral wrt $\gamma$ which can also be obtained in the nominator by shifting $\zeta_\rho^2$.
A maximum of this can be factorized for an appropriate choice of $\rho$.
\\
}
